# Supplementary material for: Ising model close to $d=2$
Source: arXiv:2107.13679 source file (2022-05-12)
Supplement: Supplementary file 1 [file Ising_2+eps_supplemental-material.pdf]

# Supplemental Material for “The $\epsilon = d - 2$ expansion of the Ising model”

Wenliang Li\*

*School of Physics, Sun Yat-Sen University, Guangzhou 510275, China and  
Okinawa Institute of Science and Technology Graduate University, 1919-1 Tancha, Onna-son, Okinawa 904-0495, Japan*

We present some explicit formulas relevant to the analytical bootstrap approach.

## I. EXPLICIT EXPRESSIONS OF $|\Delta_\sigma\rangle$ AND $|d\rangle$

To perform the analytical study of the crossing equation, we need to know the explicit expressions of various terms. The case of  $|\Delta_\sigma\rangle$  is simple:

$$|\Delta_\sigma\rangle = \frac{\sqrt{1 + \sqrt{u} + \sqrt{v}}}{\sqrt{2}} \log v - (z \leftrightarrow 1 - \bar{z}). \quad (1)$$

The definition of  $|d\rangle$  is

$$|d\rangle = \sum_i v^{\frac{1}{8}} (\lambda_{\tau_i, \ell_i}^{(0)})^2 \partial_d G_{\tau_i, \ell_i}^{(d)}(z, \bar{z}) \Big|_{d \rightarrow 2} - (z \leftrightarrow 1 - \bar{z}). \quad (2)$$

We can divide the sum over spin into a low spin part and a high spin part. The low spin contributions to the regular terms can be computed exactly in the small  $1 - \bar{z}$  expansion. For the high spin part, we first use the large spin expansion of the 2d data to compute the exact singular terms to high order, such as  $(1 - \bar{z})^{40-1/8}$ . Then we use the  $SL(2, \mathbb{R})$  resummation identities to evaluate the regular terms and compute the full regular terms to high precision. In this way, we can compute the contribution of a twist trajectory order by order in  $z, 1 - \bar{z}$

$$\sum_\ell (\lambda_{\tau, \ell}^{(0)})^2 \partial_d G_{\tau, \ell}^{(d)}(z, \bar{z}) \Big|_{d \rightarrow 2} = \sum_{n=1}^{\infty} z^{\tau/2+n} \left( D_{\tau, n}^{(s)}(1 - \bar{z}) + D_{\tau, n}^{(r)}(1 - \bar{z}) \right), \quad (3)$$

which encodes the contributions with identical twist. Here  $D^{(s)}$  and  $D^{(r)}$  denote singular and regular terms, which have finite and vanishing double discontinuities, respectively. Note that the double discontinuity is defined by analytical continuation around the branch point  $\bar{z} = 1$ . The  $n$  summation starts from  $n = 1$  because the  $n = 0$  part is independent of  $d$ . One can also see that the conformal blocks in  $d = 2$  and  $d = 2 + \epsilon$  dimensions are linear independent.

Below we will present the explicit results that are relevant to our analysis near the double lightcone limit. The leading terms of the singular part are

$$D_{0,1}^{(s)}(x) = \left( \frac{1}{4} + \frac{1}{8} x^{\frac{1}{2}} - \frac{23}{224} x^1 + \frac{59}{704} x^{\frac{3}{2}} - \frac{37}{512} x^2 + \dots \right) \frac{x^{-\frac{1}{8}}}{\sqrt{2}}, \quad (4)$$

$$D_{0,2}^{(s)}(x) = \left( \frac{1}{8} + \frac{1}{16} x^{\frac{1}{2}} - \frac{39}{448} x^1 + \frac{107}{1408} x^{\frac{3}{2}} - \frac{1291}{15360} x^2 + \dots \right) \frac{x^{-\frac{1}{8}}}{\sqrt{2}}, \quad (5)$$

$$D_{1/2,1}^{(s)}(x) = \left( \frac{1}{8} - \frac{1}{16} x^{\frac{1}{2}} + \frac{95}{3136} x^1 - \frac{905}{15488} x^{\frac{3}{2}} + \frac{177881}{3763200} x^2 + \dots \right) \frac{x^{-\frac{1}{8}}}{\sqrt{2}}. \quad (6)$$

We only give the exact results to order  $x^2$ , but they have been computed to high order, such as order  $x^{20}$ . To order  $z^2$ , the above results are sufficient, but we have also computed the explicit expressions with higher  $\tau$  and  $n$ , which are of higher order than  $z^2$ . The regular terms can also be computed order by order to high precision

$$D_{0,1}^{(r)}(x) = -\frac{3}{16G}, \quad (7)$$

\* liwliang3@mail.sysu.edu.cn

$$D_{0,2}^{(r)}(x) \approx -0.10471666 + \frac{1}{128} \log(1-x) + \frac{1}{256} \log x, \quad (8)$$

$$D_{1/2,1}^{(r)}(x) \approx 0.06743304 + 0.02179289 x + 0.00814652 x^2 + \dots \\ + 0.00986926 \left(1 - \frac{1}{4}x - \frac{7}{64}x^2 + \dots\right) \log x, \quad (9)$$

where  $G = \Gamma(1/4)^2 (2\pi)^{-3/2}$  is Gauss's constant. We only write the numerical coefficients to precision  $10^{-8}$ , but they have been evaluated at much higher precision. The exact coefficients were guessed from the high-precision numerical values and we have checked that they are consistent with the direct summation over spin. For example, we first computed  $D_{0,1}^{(r)}$  to precision  $10^{-50}$  using the large spin expansion and  $SL(2, \mathbb{R})$  resummation identities and guessed the analytic expression. Then we verified that the direct summation from  $\ell = 0$  to  $\ell = 40476 \approx 2^7 \times 10^{5/2}$  matches  $D_{0,1}^{(s)}(x) + D_{0,1}^{(r)}(x)$  at  $x = 10^{-5}$  with precision  $10^{-100}$ .

Let us also provide the leading bi-singular terms of  $|d\rangle$

$$|d\rangle_{\text{b.s.}} = \frac{1}{4\sqrt{2}} \left( z - (1 - \bar{z}) \right) + \frac{1}{8\sqrt{2}} \left( \sqrt{z} - \sqrt{1 - \bar{z}} \right) \left( \sqrt{z} + \sqrt{1 - \bar{z}} \right)^2 \\ + \frac{1}{32\sqrt{2}} \left( \sqrt{z} - \sqrt{1 - \bar{z}} \right) \left( \sqrt{z} + \sqrt{1 - \bar{z}} \right) \left( 3z - 2\sqrt{z}\sqrt{1 - \bar{z}} + 3(1 - \bar{z}) \right) \\ + \frac{1}{256\sqrt{2}} \left( \sqrt{z} - \sqrt{1 - \bar{z}} \right) \left( 23z^2 + 35z^{3/2}(1 - \bar{z})^{1/2} + \frac{11481}{1078} z(1 - \bar{z}) + (z \leftrightarrow 1 - \bar{z}) \right) \\ + \dots, \quad (10)$$

which are determined by the asymptotic behaviour of the 2d OPE coefficients at large spin.
